# Supplementary material for: CorpusVis: Visual Analysis of Digital Sheet Music Collections
Source: arXiv:2203.12663 source file (2022-03-23)
Supplement: Supplementary file 1 [file 99_appendix.tex]

\appendix

\section*{Appendix}

\section{Terminology} \label{sec:terminology}

Chords, Fakebook, Sheet music, chord symbols, musical scores, visual representation of auditory information.

Conductor scores (grouping of instruments) 

Handwritten, vs. printed, vs. digital format that can be visualized in different ways.. Digital sheet music formats shape the way how sheet music is organized

Information that is encoded in sheet music is \cite{Miller2018}.
Jazz music only chords, no melody encoded but rather improvisation.

Focus of sheet music: what features are analyzed?

traditional/classic vs. popular music 

score is an alternative term for sheet music

Scores typically contain the following information: who is the composer, if arranged (by who arranged?). general issue of copyright?

copyright is a problem that marginalizes existing composers, which data can be easily accessed. 

Low-level features — based on musical data, we can extract low-level feature information that describes a very specific aspect of a composition in a rather summarized way.

\section{Detailed Dataset Characteristics} \label{app:datasetCharacteristics}

The dataset that contains a musical score corpus of 10851 compositions from. 
In total, 1918 different composers and 128 composers with more than 10 compositions. In the composer timeline of the data selection and filtering component, only 62 of the 128 composers are listed, because only for these composers were at least one composition in the dataset that provided the lifetime period of the respective composer.

Twenty-nine different types/styles/genres ?! are considered that are ordered by average composing date ordered chronically on the horizontal axis: 
"soundtrack", "medley", "nocturne", "ballad", "chorale", "hymn", "concerto", "minuet", "prelude", "lauda", "scherzo", "fantasia", "requiem", "oratorio", "sonata", "intermezzo", "symphony", "etude", "serenade", "rondo", "opera", "suite", "fugue", "rhapsody",waltz", "mazurka", "madrigal", "polonaise"
